# Supplementary material for: STEP: Enhancing Video-LLMs' Compositional Reasoning by Spatio-Temporal Graph-guided Self-Training
Source: arXiv:2412.00161 source file (2025-03-30)
Supplement: Supplementary file 1 [file X_suppl.tex]

\clearpage
\setcounter{page}{1}
\setcounter{section}{0}
\maketitlesupplementary

\section*{Overview}
\noindent In this supplementary material, we present:
\begin{itemize}
    \item The detailed prompt for STSG construction and QRA refinement (Section \ref{sec:A})
    \item The specifics of the backbone models (Section \ref{sec:B})
    \item Implementation details (Section \ref{sec:C})
    \item The evaluation details for each datasets (Section \ref{sec:D})
    \item Additional experimental results (Section \ref{sec:E})
    \item More Qualitative Visualizations (Section \ref{sec:F})
\end{itemize}
\section{Detailed Prompt Design}
\label{sec:A}
\subsection{Prompt for STSG Construction}
Here, we provide detailed prompts as well as their inputs and outputs, for each step of the STSG Construction.
\subsubsection*{Semantics Parsing}

\specialtitle{Step-1}: For each keyframe, first get its scene narrative, then extract the object information.

% 灰色大框
\begin{tcolorbox}[colframe=grey!80, colback=gray!10, coltitle=black, title=Step-1: Object Nodes Parsing, breakable]

% 输入部分
\textbf{{$\blacktriangleright$ Input1:}}

$[$ INST $]$

Describe the keyframe of the video in one sentence, ensuring to include all main objects within the scene.

$[$ /INST $]$

$<$Image$>$
\includegraphics[width=0.08\linewidth]{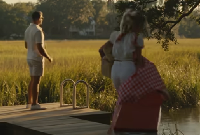}
$<$/Image$>$

\vspace{1em}

% 输出部分
\textbf{\textcolor{black}{$\blacktriangleright$ Output1:}}
\texttt{[In the keyframe, a man and a woman carrying a red box are on a dock.]}

\vspace{1em}

\textbf{{$\blacktriangleright$ Input2:}}

$[$ INST $]$

From the given sentence, the task is to extract meaningful objects. Note that the object is the entity or noun that being described in the sentence.
Let's take a few examples to understand how to extract meaningful objects.

Question: Given the sentence “Children play with red toys in the yard,” extract meaningful objects. Answer: Meaningful objects are [children, toys, yard].

Question: Given the sentence “A beautiful woman walking a dog on top of a beach,” extract meaningful objects. 

Answer: Meaningful objects are [woman, dog, beach].

Question: Given the sentence ``A mix of black and white cat jumps over a old fence," extract meaningful objects. 

Answer: Meaningful objects are [cat, fence].  

Please answer the following question. 

Question: Given the sentence ``\texttt{[A man and a woman carrying a red box are on a dock]}," extract meaningful objects. 

Answer: 

$[$ /INST $]$

\vspace{1em}

\textbf{{$\blacktriangleright$ Output2:}}

\texttt{[Meaningful objects are [man, woman, box, dock].]}

\vspace{1em}

\textbf{{$\blacktriangleright$ Input3:}}

$[$ INST $]$

Given the object name: \texttt{[man]}, if there is more than one, please provide the quantity and describe each instance of \texttt{[man]} with a corresponding unique attribute. The unique attribute should be something that only one instance has while the others do not. Use the following format for the output:

Object:  \texttt{[man]} \\
Quantity: [number] \\
1. \texttt{[man]}1: [distinct unique attribute] \\
2. \texttt{[man]}2: [distinct unique attribute] \\
... \\
$[$ /INST $]$

$<$Image$>$
\includegraphics[width=0.08\linewidth]{fig/fig.png}
$<$/Image$>$
\vspace{1em}

\textbf{{$\blacktriangleright$ Output3:}}

\texttt{[Object: man \\
Quantity: 1 \\
1. man1: wearing a light-colored shirt and shorts]}

\vspace{1em}

\textbf{{$\blacktriangleright$ Input4:}}

Given the object: \texttt{[man]}, determine if it is a static object or a dynamic object. 
Note that static objects refer to background objects that may not move or change observably within a short time while dynamic objects are the opposite.
If the object is static, print `Static', otherwise print `Dynamic', no explanation is needed.
\vspace{0.5em}

$<$Video$>$
\includegraphics[width=0.09\linewidth]{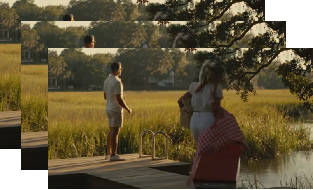}
$<$/Videos$>$

\vspace{1em}

\textbf{{$\blacktriangleright$ Output4:}}
\texttt{[Dynamic]}

\end{tcolorbox}

\specialtitle{Step-2}: For each object, we request a detailed narrative to extract its fine-grained attributes.

\begin{tcolorbox}[colframe=gray!80, colback=gray!10, coltitle=black, title=Step-2: Attribute Nodes Parsing, breakable]

% 输入部分
\textbf{{$\blacktriangleright$ Input1:}}

$[$ INST $]$
Given the object: \texttt{[man]}, describe its attributes in the scene using one or two sentences that primarily include adjectives or present participles (-ing forms). Avoid any irrelevant details or complex explanations.

$[$ /INST $]$

$<$Image$>$
\includegraphics[width=0.08\linewidth]{fig/fig.png}
$<$/Image$>$

\vspace{1em}

% 输出部分
\textbf{\textcolor{black}{$\blacktriangleright$ Output1:}}
\texttt{[The man is standing on a wooden dock, wearing a white shirt and gray 
shorts and looking out over a serene marshy area.]}

\vspace{1em}

\textbf{{$\blacktriangleright$ Input2:}}

$[$ INST $]$

For the given sentence, the task is to extract meaningful attributes for the given object. Each attribute should include its type and value. Let's take a few examples to understand how to extract meaningful attributes.

Question: Given the sentence “A woman with long and blonde hair is sitting on a park bench,” extract meaningful attributes for the object “woman”. 

Answer: [“object”:“woman”, “attributes":[“hair”:
“long and blonde”, “status”:“sitting”]]   

Question: Given the sentence ``A tall man in a red jacket is walking down the street," extract meaningful attributes for the object ``man".

Answer: [``object":``man", ``attributes":[``height":
``tall", ``clothing":``red jacket", ``action":
``walking"]]

Question: Given the sentence ``The blue car is parked," extract meaningful object label and attributes for the object ``car"

Answer: [``object":``car", ``attributes":[``color":``bl-
ue", ``status":``parked"]]

Please answer the following question. 

Question: Given the sentence ``\texttt{[The man is standing on a wooden dock, wearing a white shirt and gray shorts and looking out over a serene marshy area]}."  Extract meaningful attributes for the object “\texttt{[man]}”

Answer:

$[$ /INST $]$

\vspace{1em}

\textbf{{$\blacktriangleright$ Output2:}}

\texttt{[["object":"man", "attributes":
["clothing":"white shirt", 
"clothing":"gray shorts", "status":"standing"]]]}

\end{tcolorbox}

\specialtitle{Step-3}: For each pair of object nodes, we construct $<$ subject,predicate,object $>$ triples to capture their relational correspondence.

\begin{tcolorbox}[colframe=gray!80, colback=gray!10, coltitle=black, title=Step-3: Relation Edges Parsing, breakable]

% 输入部分
\textbf{{$\blacktriangleright$ Input1:}}

$[$ INST $]$

Given the object: \texttt{[man]} in the provided image, describe all spatial or contact relationship between \texttt{[man]} and other objects \texttt{[woman, dock, box]} in the image. Ensure the subject of every sentence is \texttt{[man]}, and do not include detailed descriptions of other objects.

$<$Image$>$
\includegraphics[width=0.08\linewidth]{fig/fig.png}
$<$/Image$>$

$[$ /INST $]$

\vspace{1em}

\textbf{{$\blacktriangleright$ Output1:}}

\texttt{[The man is standing at the end of a dock, waiting for the woman.]}

\vspace{1em}

\textbf{{$\blacktriangleright$ Input2:}}

$[$ INST $]$
From the given sentence, the task is to extract meaningful triplets formed as $<$subject, predicate, object$>$. Note that the subject must be the given object, and the object is the entity or noun that is affected by the action or is receiving the action. The predicate is a verb or adjective without auxiliary verb, and is represented without the tense (e.g., are, being). 
Let's take a few examples to understand how to extract meaningful triplets. 

Question: Given the sentence ``a slice of bread is covered with a sour cream and quacamole," extract meaningful triplets for the given object ``bread". 

Answer: Meaningful triplets are $<$bread, covered with, sour cream$>$, $<$bread, covered with, guacamole$>$. 

Question: Given the sentence ``A clock sitting on a floor next to a woman's feet," extract meaningful triplets for the given object ``clock". 

Answer: Meaningful triplets are $<$clock, sitting on, floor$>$, $<$clock, next to, feet$>$. 

Question: Given the sentence ``One person sits in a chair looking at her phone while another rests on the couch," extract meaningful triplets for the given object ``person". 

Answer: Meaningful triplets are $<$person, sits in, chair$>$, $<$person, looking at, phone$>$, $<$person, rests on, couch$>$. 

Please answer the following question.

Question: Given the sentence ``\texttt{[The man is standing at the end of a dock, waiting for the woman]}," extract meaningful triplets for the given object \texttt{[man]}.

Answer:

\vspace{1em}
\textbf{{$\blacktriangleright$ Output2:}}

\texttt{[Meaningful triplets are $<$man, standing at, the end of dock$>$, $<$man, waiting for, woman$>$]}

\end{tcolorbox}

\specialtitle{Verification}: Filter the hallucinated nodes.

\begin{tcolorbox}[colframe=gray!80, colback=gray!10, coltitle=black, title=Step-1: Identify the Cross-frame Object Nodes,breakable]

% 输入部分
\textbf{{$\blacktriangleright$ Input1:}}

$[$ INST $]$

For the given video, determine if \texttt{[the box whose color is red]} truly exists in the given video. 

$[$ /INST $]$

$<$Video$>$
\includegraphics[width=0.09\linewidth]{fig/video.png}
$<$/Videos$>$

\vspace{1em}

\textbf{{$\blacktriangleright$ Output1:}}
\texttt{[Yes]}

\end{tcolorbox}

\vspace{1em}
\subsubsection*{Dynamic Merging}

\specialtitle{Step-1}: Determine if the nodes in different keyframes are identical.

\begin{tcolorbox}[colframe=gray!80, colback=gray!10, coltitle=black, title=Step-1: Identify the Cross-frame Object Nodes,breakable]

% 输入部分
\textbf{{$\blacktriangleright$ Input1:}}

$[$ INST $]$

For the given video, determine if \texttt{[woman walking on the dock
]} in the first half and \texttt{[woman kneeling on the dock]} in the second half are the same object. Just output `Yes' or `No'.

$[$ /INST $]$

$<$Video$>$
\includegraphics[width=0.09\linewidth]{fig/video.png}
$<$/Videos$>$

\vspace{1em}

\textbf{{$\blacktriangleright$ Output1:}}
\texttt{[Yes]}

\end{tcolorbox}

\specialtitle{Step-2}: If the two identical object nodes are static, just merge them into a single unified node, dynamic, the prompt should be:

\begin{tcolorbox}[colframe=gray!80, colback=gray!10, coltitle=black, title=Step-2: Connect the Dynamic Nodes, breakable]
\textbf{{$\blacktriangleright$ Input1:}}

Given the same object \texttt{[woman walking on the dock]} in the first half video and \texttt{[woman kneeling on the dock]}
in the second half video, describe the action of this object in the video.
\vspace{1em}

\textbf{{$\blacktriangleright$ Output1:}}
\texttt{[The woman fell down on the dock.]}

\vspace{1em}

\textbf{{$\blacktriangleright$ Input2:}}

For the given sentence, the task is to extract meaningful action for the given object. The action should be described using a verb or verb phrase.
Let's take a few examples to understand how to extract.

Question: Given the sentence ``The man walked on the street," extract meaningful action for the object ``man".

Answer: [``action":``walking on the street"]

Question: Given the sentence ``The cat jumped on the bed," extract meaningful action for the object ``cat".

Answer: [``action":``jumping on the bed"]

Question: Given the sentence "The dog chased the ball in the park," extract meaningful action for the object "dog".

Answer: ["action": "chasing the ball in the park"]

Please answer the following question.

Question: Given the sentence ``\texttt{[The woman fell down on the dock]}," extract meaningful action for the object ``\texttt{[woman]}".

Answer:

\vspace{1em}
\textbf{{$\blacktriangleright$ Output2:}}

\texttt{[["action":"falling down on the dock"]]}

\vspace{1em}
\textbf{{$\blacktriangleright$ Input3:}}

For the given action, extract the predicate and object. The predicate is a verb or verb phrase, and the object is the entity or noun that is affected by the action.
Let's take a few examples to understand how to extract.

Question: Given the action ``walking", extract the predicate and object.

Answer: [``predicate":``walking", ``object"
:``None"]

Question: Given the action ``jumping on the bed", extract the predicate and object.

Answer: [``predicate":``jumping on", ``object":
``bed"]

Question: Given the action ``sitting on the chair", extract the predicate and object.

Answer: [``predicate":``sitting on", ``object":
``chair"]

Please answer the following question.

Question: Given the action ``\texttt{[falling down on the dock]}", extract the predicate and object.

Answer:

\vspace{1em}
\textbf{{$\blacktriangleright$ Output3:}}

\texttt{[["predicate":"falling down on", "object":"dock"]]}
\end{tcolorbox}

\vspace{1em}

\subsubsection*{Cross-clip Bridging}

\specialtitle{Step-1}: Determine if the nodes in different clips represent the same object. If they do, connect them with a reference edge.

\begin{tcolorbox}[colframe=gray!80, colback=gray!10, coltitle=black, title=Step-1: Identify the Cross-clip Object Nodes,breakable]

% 输入部分
\textbf{{$\blacktriangleright$ Input1:}}

$[$ INST $]$

For the given video, determine if \texttt{[woman walking on the dock
]} in the first clip and \texttt{[woman sitting on the blanket]} in the second clip are the same object. Just output `Yes' or `No'.

$[$ /INST $]$

$<$Video$>$
\includegraphics[width=0.09\linewidth]{fig/video.png}
$<$/Videos$>$

\vspace{1em}
\textbf{{$\blacktriangleright$ Output1:}}

\texttt{[Yes]}

\end{tcolorbox}

\vspace{1em}
\subsection{Prompt for QRA refinement}

\begin{tcolorbox}[colframe=gray!80, colback=gray!10, coltitle=black, title=Step-1: Identify the Object Nodes,breakable]

% 输入部分
\textbf{{$\blacktriangleright$ Input1:}}

$[$ INST $]$

I have the question ``\texttt{[q]}", the rationale ``\texttt{[r]}", and the answer ``\texttt{[a]}" about the video.
Due to template generation, these may contain grammatical errors, logical inconsistencies, or unclear semantics. 
Please correct them and return the improved version in JSON format : \{``Q": ``question", ``R": ``rationale", ``A": ``answer"\}

$[$ /INST $]$

\end{tcolorbox}

\section{Backbone Models Specifications}
\label{sec:B}
\subsection{VideoChat2 (7B)}
VideoChat2 is an advanced Video-LLM designed to handle complex video-language understanding tasks \cite{li2024mvbench}. Its architecture integrates a visual encoder, a Q-Former module for compressing and aligning visual data, and a large language model (LLM) for advanced reasoning and response generation. The training process follows a progressive three-stage paradigm: vision-language alignment to link visual and textual features, vision-language connection to integrate visual embeddings with the LLM, and instruction tuning to enhance multi-modal instruction-following capabilities.

The version we use is VideoChat2 with Mistral 7B. To endow the initial model with a baseline level of instruction-following capability, we selected 60K samples from the instruction-tuning dataset of VideoChat2 for foundational instruction tuning on the pre-trained (vision-language aligned) VideoChat2 model, which results in VideoChat2*. The details are presented in Table \ref{tab:table5}.
\setlength{\tabcolsep}{4pt}
\begin{table}[h]
    \centering
    \begin{tabularx}{\linewidth}{c|l|l|c}
        \toprule
        Modality & Dataset & Description & \# Samples  \\
        \midrule
        \multirow{2}{*}{Image-Text} & CoCo
         & Captioning & 5K \\
        & VQAv2 & General & 10K  \\
        \midrule
        \multirow{6}{*}{Video-Text} & VideoChat & Captioning & 5K  \\
        & SthSthV2 & Classification & 5K \\
        & VideoChatGPT & General & 10K\\
        & NExTQA & Reasoning & 10K \\
        & CLEVRER & Reasoning & 5K  \\
        & Tgif & Reasoning & 10K  \\
        \bottomrule
        Total & &  & 60K \\
        \end{tabularx}
    \caption{Data mixture of initial instruction tuning}
    \label{tab:table5}
\end{table}

\subsection{VILA (3B)}
VILA is a Video-LLM evolved from an Image-LLM \cite{lin2024vila}. It employs an autoregressive architecture that integrates tokenized images with text inputs. The training process includes three stages: projector initialization for modality alignment, visual-language pre-training on interleaved datasets to enhance zero-shot and in-context learning, and visual instruction-tuning to optimize task-specific performance.
In the instruction-tuning stage, VILA incorporates video-based instruction datasets, extending its capabilities to spatio-temporal reasoning as a lightweight Video-LLM.

Since VILA does not provide checkpoints after the visual-language pre-training stage, we are unable to perform instruction-tuning with a small amount of data. Instead, we directly use the fully instruction-tuned model as the initial model in our \textbf{STEP} framework.

\section{Implementation Details}
\label{sec:C}
\textbf{STEP} method first constructs STSGs for diverse videos in the raw video datasets during the symbolic structure induction phase. It then utilizes stepwise graph-driven rationale learning to systematically extract reasoning-rich training data and perform explicit supervision for the reasoning process. This process is iterative rather than a one-step procedure, to better leverage the model’s enhanced capabilities in each cycle, enabling progressive improvement in reasoning through repeated data generation and training, ultimately forming a self-enhancing closed-loop mechanism.

We selected three video datasets: ActivityNet \cite{caba2015activitynet}, Ego4D \cite{grauman2022ego4d}, and Charades \cite{sigurdsson2018charades} as the raw video sources. ActivityNet tracks human actions in videos, Ego4D captures life from a first-person perspective, and Charades records home-based daily tasks. The diversity in video nature—ranging from third-person action tracking to first-person experiences and everyday household activities—demonstrates how \textbf{STEP} can effectively adapt to different contexts, enabling robust symbolic structure induction and reasoning across a broad spectrum of real-world scenarios. The total number of QRAs extracted from these three raw video datasets is as follows:

\begin{table}[h]
    \centering
    \begin{tabular}{l|c}
        \toprule
        Raw Video Sources & \# QRA Samples  \\
        \midrule
        ActivityNet & 15K \\
        Ego4D & 5K \\
        Charades & 10K \\
        \bottomrule
        Total & 30K \\
        \end{tabular}
    \caption{Number of QRAs extracted from three raw video datasets}
    \label{tab:table6}
\end{table}

For the \textbf{STEP} model, we perform explicit rationale supervision using the derived QRA training samples. Additionally, to mitigate catastrophic forgetting and enhance overall video comprehension, the training data is augmented by incorporating previously utilized instruction-tuning data from VideoChat* and VILA, with \( L_{rationale} = 0 \) to retain only \( L_{answer} \) for these datasets. 

For the \textit{Instruct} model, we utilize the annotated labels from the same video datasets—ActivityNet, Ego4D, and Charades—to generate a annotated training set. The number of QA samples is the same as Table \ref{tab:table6}. Since these traditional
datasets only contain questions and answers, conventional
training is applied with $L_{rationale}$ = 0, focusing solely on
answer-based supervision.

For the \textit{Distillation} model, the raw videos and training sample size are consistent with those used for the \textbf{STEP} model, ensuring that the distillation process is based on the same foundational data.
\section{Evaluation Details}
\label{sec:D}

For the compositional reasoning benchmarks AGQA \cite{grunde2021agqa} and STAR \cite{wu2024star}, and the standard QA datasets MSVD-QA \cite{xu2017video}, MSRVTT-QA \cite{xu2016msr}, and ActivityNet-QA \cite{caba2015activitynet}, we apply the same evaluation protocol as  \cite{achiam2023gpt}, which reports two key metrics: accuracy (the percentage of correctly answered questions) and the average score (where ChatGPT rates each response on a scale of 1-5 and calculates the mean of these scores). To ensure consistent comparisons, all evaluations utilize the same GPT model, ``gpt-3.5-turbo" \cite{wu2024freeva}. All evaluation prompt is ``Based on the video, respond to this question with a short answer: \{question\}".

For the comprehensive understanding benchmarks MVBench \cite{li2024mvbench} and TempCompass \cite{liu2024tempcompass}, the long video understanding benchmarks MovieChat-1K \cite{song2024moviechat} and MLVU \cite{zhou2024mlvu}, we adhere strictly to the evaluation methodologies specified in their respective frameworks. 

Across all evaluations, each video is represented by 8 frames as input, with a resolution of \(224 \times 224\). This setup ensures consistency in video processing and facilitates a fair comparison of model performance across diverse benchmarks.
\begin{table}[h]
\centering
\label{tab:table7}
\begin{tabularx}{\linewidth}{@{}c|l|c|c@{}}
\toprule
Type & Dataset & Split & Metrics \\ \midrule
Compositional & AGQA & test & Accuracy, Score   \\
Reasoning & STAR & val & Accuracy, Score  \\
\midrule
\multirow{3}{*}{Standard QA} & MSVD-QA & test & Accuracy, Score  \\
& MSRVTT-QA  & test & Accuracy, Score \\
& ActivityNet-QA & test & Accuracy, Score \\
\midrule
Comprehensive& TempCompass & - & VQA Accuracy  \\ 
Understanding& MVBench & - &  VQA Accuracy  \\
\midrule
Long video& MovieChat-1K  & - & Accuracy, Score\\ 
Understanding& MLVU & - &  VQA Accuracy  \\
\bottomrule
\end{tabularx}
\caption{Evaluation metrics for each evaluation benchmarks}
\end{table}

\setlength{\tabcolsep}{3.5pt} 
\begin{table*}[t]
\centering
\begin{tabular}{lccccccccccccc}
\toprule
\textbf{Method} & \multicolumn{2}{c}{\textbf{Action}} & \multicolumn{2}{c}{\textbf{Direction}} & \multicolumn{2}{c}{\textbf{Speed}} & \textbf{Event} & \multicolumn{4}{c}{\textbf{Attribute Change}} & \textbf{Avg} \\
\cmidrule(lr){2-3} \cmidrule(lr){4-5} \cmidrule(lr){6-7} \cmidrule(lr){8-8} \cmidrule(lr){9-12}
& fine & coarse & object & camera & absolute & relative & order & color & size & combined & other & \\
\midrule
Random & 28.4 & 29.3 & 28.3 & 26.3 & 30.6 & 33.0 & 32.2 & 30.1 & 28.9 & 26.4 & 25.9 & 29.9 \\
VideoChatGPT(7B) & 28.8 & 62.2 & 33.7 & 26.1 & 28.2 & 28.5 & 37.1 & 26.9 & 31.1 & 35.0 & 33.3 & 35.2 \\
Video-LLaVA(7B)& 54.9 & 83.2 & 31.7 & 33.7 & 46.0 & 33.2 & 41.4 & 39.7 & 40.2 & 35.0 & 55.6 & 44.7 \\
\midrule
VideoChat2(7B)* & 73.9 & 90.8 & 37.4 & 45.7 & 54.8 & 32.6 & 37.7 & 34.6 & 42.4 & 46.7 & 27.8 & 49.0 \\
VideoChat2* $Instruct$  & 82.4 & 95.6 & 37.4 & 44.8 & 54.8 & 35.3 &  40.7 &  43.6 &  42.4 & 45.0 & 38.9 & 51.8\\
VideoChat2* $Distillation$ & 84.0 & 94.8 & 40.7 & 43.3 & 58.9 & 34.2 & 43.1 & 48.7 & 44.8 & 50.7 & 38.8 & 53.6 \\
VideoChat2* \textbf{STEP} & 85.7 & 95.7 & 41.2 & 43.5 & 60.1 & 33.7 & 46.4 & 51.3 & 51.5 & 53.5 & 38.9 & 55.4\\
\midrule
VILA(3B) & 74.3 & 93.5 & 33.7 & 37.0 & 52.4 & 41.9 & 40.4 & 62.8 & 46.2 & 38.7 & 50.0 & 51.4 \\
VILA $Instruct$  & 78.9 & 94.8 & 34.8 & 38.9 & 47.8 & 43.2 & 39.7 &  65.7 & 51.5 & 38.9 & 51.7 & 52.6\\
VILA $Distillation$ & 80.4 & 94.8 & 37.0 & 38.0 & 50.2 & 36.8 & 43.0 & 74.8 & 50.0 & 41.0 & 51.6 & 53.5 \\
VILA \textbf{STEP} & 83.0 & 95.7 & 38.0 & 40.2& 47.8 & 34.2 & 43.4 & 78.2& 56.8 & 41.0 & 52.1& 54.4 \\
\bottomrule
\end{tabular}
\captionsetup{font=normalsize} 
\vspace{-0.5em}
\caption{Model performance comparison on multi-choice QA for TempCompass on VideoChat2* and VILA}

\label{tab:multi_choice_qa}
\end{table*}

\setlength{\tabcolsep}{3.5pt} 
\begin{table*}[t]
\centering
\begin{tabular}{lccccccccccccc}
\toprule
\textbf{Method} & \multicolumn{2}{c}{\textbf{Action}} & \multicolumn{2}{c}{\textbf{Direction}} & \multicolumn{2}{c}{\textbf{Speed}} & \textbf{Event} & \multicolumn{4}{c}{\textbf{Attribute Change}} & \textbf{Avg} \\
\cmidrule(lr){2-3} \cmidrule(lr){4-5} \cmidrule(lr){6-7} \cmidrule(lr){8-8} \cmidrule(lr){9-12}
& fine & coarse & object & camera & absolute & relative & order & color & size & combined & other & \\
\midrule
Random & 50.0 & 50.0 & 50.0 &50.0 & 50.0 & 50.0 & 50.0 & 50.0 & 50.0 & 50.0 & 50.0 & 50.0 \\
VideoChatGPT(7B) & 50.2 &54.5& 50.0& 50.0 &49.7 &49.4 &51.0 &50.0 &50.0& 50.0 &50.0 &50.7 \\
Video-LLaVA(7B)& 58.4 & 87.6 &51.4 &52.7& 50.8 &50.0 &49.2 &52.2 &50.0 &53.0 &45.8 &56.4 \\
\midrule
VideoChat2(7B)* & 57.6 & 89.2 & 50.3 & 50.7 &  65.1 & 49.4 & 53.4 & 55.9 & 52.1 & 54.0 &  50.0 & 58.3 \\
VideoChat2* $Instruct$  &  58.0 &  90.4 & 53.5 & 50.0 & 66.4 & 49.1 &  53.6 &  58.1 &  53.7 & 56.0 & 50.0 & 59.4\\
VideoChat2* $Distillation$ & 59.2 & 91.6 & 53.5 & 52.1 & 68.3 & 51.1 & 54.0 & 58.6 & 54.8 & 57.0 & 49.8 & 60.4 \\
VideoChat2* \textbf{STEP} 60.1 & 91.7 & 52.9 & 52.0 & 68.1 & 51.3 & 56.4 & 59.3& 54.5 & 57.7 & 50.3 & 60.9 \\
\midrule
VILA(3B) & 65.8 & 87.4 & 52.3 & 52.7 & 52.9 & 50.6 & 54.2 & 63.2 & 61.2 & 56.0 & 62.5 & 60.1 \\
VILA $Instruct$  &  67.8 & 90.5 & 52.1 & 53.0 & 53.2 & 54.2 & 55.4 & 63.8 & 64.7 & 57.3 & 62.9 & 61.8\\
VILA $Distillation$ & 68.3 & 91.5 & 53.2 & 52.9 & 53.8 & 53.7 & 55.9 & 64.7 & 65.0 & 58.6 & 63.5 & 62.3 \\
VILA \textbf{STEP} & 69.1 &91.7& 53.6 & 53.0 & 53.7 & 53.9& 56.4 & 65.3 & 65.5 &59.2 & 63.9 & 62.7 \\
\bottomrule
\end{tabular}
\captionsetup{font=normalsize} 
\vspace{-0.5em}
\caption{Model performance comparison on yes/no QA for TempCompass on VideoChat2* and VILA}

\label{tab:yes_no_qa}
\vspace{-1em}
\end{table*}
\section{Additional Experimental Results}
\label{sec:E}
\subsection{TempCompass}
The TempCompass benchmark \cite{liu2024tempcompass} encompasses four task types: Multi-Choice QA, Yes/No QA, Caption Matching, and Caption Generation. The detailed results can be found in Tables  \ref{tab:multi_choice_qa}, \ref{tab:yes_no_qa}, \ref{tab:caption}.
\setlength{\tabcolsep}{1pt} 
\begin{table*}[t]
\centering
% 表格标题
\begin{tabular*}{\textwidth}{@{}l|c*{20}{|c}@{}} % 设置列格式
\toprule
\textbf{Model} & \textbf{Avg} & \textbf{AS} & \textbf{AP} & \textbf{AA} & \textbf{FA} & \textbf{UA} & \textbf{OE} & \textbf{OI} & \textbf{OS} & \textbf{MD} & \textbf{AL} & \textbf{ST} & \textbf{AC} & \textbf{MC} & \textbf{MA} & \textbf{SC} & \textbf{FP} & \textbf{CO} & \textbf{EN} & \textbf{ER} & \textbf{CI} \\ 
\midrule
Random & 27.3 & 25.0 & 25.0 & 33.3 & 25.0 & 25.0 & 33.3 & 25.0 & 33.3 & 25.0 & 25.0 & 25.0 & 33.3 & 25.0 & 33.3 & 33.3 & 25.0 & 33.3 & 25.0 & 20.0 & 30.9 \\
VideoChatGPT(7B) & 32.7 & 23.5 & 26.0 & 62.0 & 22.5 & 26.5 & 54.0 & 28.0 & 40.0 & 23.0 & 20.0 & 31.0 & 30.5 & 25.5 & 39.5 & 48.5 & 29.0 & 33.0 & 29.5 & 26.0 & 35.5 \\
VideoChat(7B) & 35.5 & 33.5 & 26.5 & 56.0 & 33.5 & 40.5 & 53.0 & 40.5 & 30.0 & 25.5 & 27.0 & 48.5 & 35.0 & 20.5 & 42.5 & 46.0 & 26.5 & 41.0 & 23.5 & 23.5 & 36.0 \\
\midrule
VideoChat2(7B)* & 47.0 & 63.5 & 47.0 & 66.5 & 43.0 & 56.0 & 51.5 & 68.0 & 35.0 & 20.0 & 32.5 & 82.5 & 38.5 & 36.5 & 54.5 & 45.0 & 51.0 & 42.5 & 28.5 & 38.0 & 39.0 \\
VideoChat2* $Inst$ & 47.9 & 64.0 & 49.0 & 68.5 & 43.0 & 58.0 & 53.5 & 68.5 & 36.5 & 22.0 & 33.5 & 83.5 & 39.0 & 36.0 & 54.5 & 46.5 & 52.0 & 42.0 & 31.0 & 38.5 & 39.5 \\
VideoChat2* $Dist$& 48.5 & 65.0 & 49.5 & 69.0 & 45.5 & 57.0 & 54.5 & 70.0 & 36.5 & 21.5 & 33.5 & 85.0 & 39.0 & 36.0 & 55.0 & 46.5 & 52.5 & 43.0 & 32.0 & 41.0 & 38.5\\
VideoChat2* \textbf{STEP} & 49.2 & 67.0 & 49.5 & 69.0 & 46.5 & 57.0 & 54.5 & 71.5 & 36.5 & 21.0 & 34.0 & 85.5 & 39.5 & 37.5 & 56.0 & 46.5 & 53.5 & 43.5 & 33.0 & 42.5 & 39.5\\
\midrule
VILA(3B) & 43.0 &  56.0 & 48.5 & 57.0 & 39.0 & 51.5 & 52.5 & 54.0 & 26.0 &27.5 & 28.0 & 74.5 & 37.0 & 30.5 & 53.5 & 39.0 & 40.0 & 47.0 & 31.5 & 37.0 & 30.0 \\
VILA $Instruct$  &  44.2 & 58.0 & 50.5 & 59.0 & 41.5 & 52.5 & 53.5 & 55.5 & 28.0 &27.5 & 29.5 & 76.5 & 38.5 & 30.0 & 53.5 & 39.0 & 41.0 & 48.0 & 32.0 & 38.5 & 32.0 \\
VILA $Distillation$ & 44.8 & 60.5& 50.5 & 60.0 & 43.5 & 54.0 & 54.5 & 55.5 & 28.5 &27.0 & 29.0 & 76.5 & 38.5 & 30.5 & 53.0 & 39.0 & 41.0 & 49.0 & 32.5 & 40.5 & 33.0 \\
VILA \textbf{STEP} & 45.6 & 60.5& 52.5 & 62.0 & 44.0 & 53.5 & 54.0 & 57.5 & 32.0 &26.5 & 30.0 & 78.5 & 39.5 & 30.0 & 53.5 & 40.0 & 42.5 & 49.0 & 33.5 & 41.5 & 32.0 \\
\bottomrule
\end{tabular*}

\footnotemark \small VideoChat2* $Inst$ refers to VideoChat2* $Instruct$, VideoChat2* $Dist$ refers to VideoChat2* $Distillation$.

\caption{Model performance comparisons on various dimensions in MVBench} 
\vspace{-1em}
\label{tab:mvbench}
\end{table*}
\begin{table}[b]
\centering
\small
\begin{tabular}{@{}lcc@{}}
\toprule
& Caption & Caption\\
& Matching & Generation \\
\midrule
Random & 50 & 30 \\
VideoChatGPT (7B) & 51.8 & 31.8 \\
Video-LLaVA(7B) &  63.7 & 34.8 \\
\midrule
VideoChat2 (7B)* & 67.9 & 45.3 \\
VideoChat2* $Instruct$ & 68.6 & 47.8 \\
VideoChat2* $Distillation$ & 69.4 & 48.5 \\
VideoChat2* STEP & 70.3 & 49.7 \\
\midrule
VILA (3B) & 65.2 & 39.1 \\
VILA $Instruct$ & 66.2 & 40.6   \\
VILA $Distillation$ & 66.7 & 40.8  \\
VILA STEP & 67.0 & 40.8 \\
\bottomrule 
\end{tabular}

% \captionsetup{font=normalsize} 
\caption{Model performance comparison on Caption Matching and Caption Generation for TempCompass on VideoChat2* and VILA.}
\label{tab:caption}
\end{table}

The results underscore that \textbf{STEP} achieves substantial advancements across all task categories in TempCompass. Specifically, in the Multi-Choice QA and Yes/No QA tasks, \textbf{STEP} exhibits superior performance in fine-grained dimensions such as fine action recognition, event order comprehension, and attribute change detection. These dimensions necessitate sophisticated spatio-temporal reasoning and a precise understanding of video semantics. Furthermore, \textbf{STEP} reduces hallucinations by incorporating multi-granular details and reasoning steps aligned with the query, enabling it to interpret complex temporal-spatial dependencies and tackle challenging reasoning tasks with greater accuracy and interpretability.

\subsection{MVBench}
MVBench \cite{li2024mvbench} is a comprehensive video benchmark designed to evaluate temporal reasoning in dynamic tasks. It includes 20 tasks that assess various temporal skills, from perception to cognition, aiming to test the real-world applicability of Video-LLMs. MVBench enhances static tasks by incorporating dynamic elements, such as transforming ``object location" into "motion direction," and uses an automated annotation pipeline to ensure fairness and accuracy. 

The performance metrics across cognitive and visual tasks are as follows: Action Sequence (AS) measures accuracy in identifying action sequences in videos. Action Prediction (AP) evaluates the model's ability to predict subsequent actions. Action Antonym (AA) assesses accuracy in distinguishing opposite actions, while Fine-grained Action (FA) gauges precision in recognizing subtle action variations. Unexpected Action (UA) tests the detection of abnormal actions. Object Existence (OE) evaluates object presence or absence recognition, and Object Interaction (OI) assesses understanding of object relationships. Object Shuffle (OS) measures object tracking through rearrangements. Moving Direction (MD) evaluates movement direction recognition, and Action Localization (AL) measures spatial-temporal action pinpointing. Scene Transition (ST) gauges setting changes recognition, Action Count (AC) tests action counting accuracy, and Moving Count (MC) focuses on counting moving objects. Moving Attribute (MA) assesses recognition of motion-related traits like speed or trajectory. State Change (SC) measures detection of object state changes, and Fine-grained Pose (FP) evaluates precise posture recognition. Character Order (CO) assesses narrative sequence recognition, Egocentric Navigation (EN) tests first-person spatial understanding, Episodic Reasoning (ER) measures episodic inference capacity, and Counterfactual Inference (CI) evaluates reasoning in hypothetical scenarios. Avg represents the average performance across tasks.

From the Table \ref{tab:mvbench}, it is evident that the \textbf{STEP} method leads to a significant improvement in the performance of MVBench for both models, particularly in tasks such as Action Sequence, Character Order, Fine-grained Action, and Episodic Reasoning. This underscores its enhanced capability in capturing and reasoning over complex spatio-temporal dependencies.

\section{More Qualitative Visualizations}
\label{sec:F}
We present additional qualitative visualizations to illustrate how \textbf{STEP} enhances spatio-temporal reasoning and fine-grained detail capture across a range of diverse scenarios, using VideoChat2* as the baseline.

\vspace{-1em}
\begin{figure}[h]
    \centering
    \includegraphics[width=\linewidth]{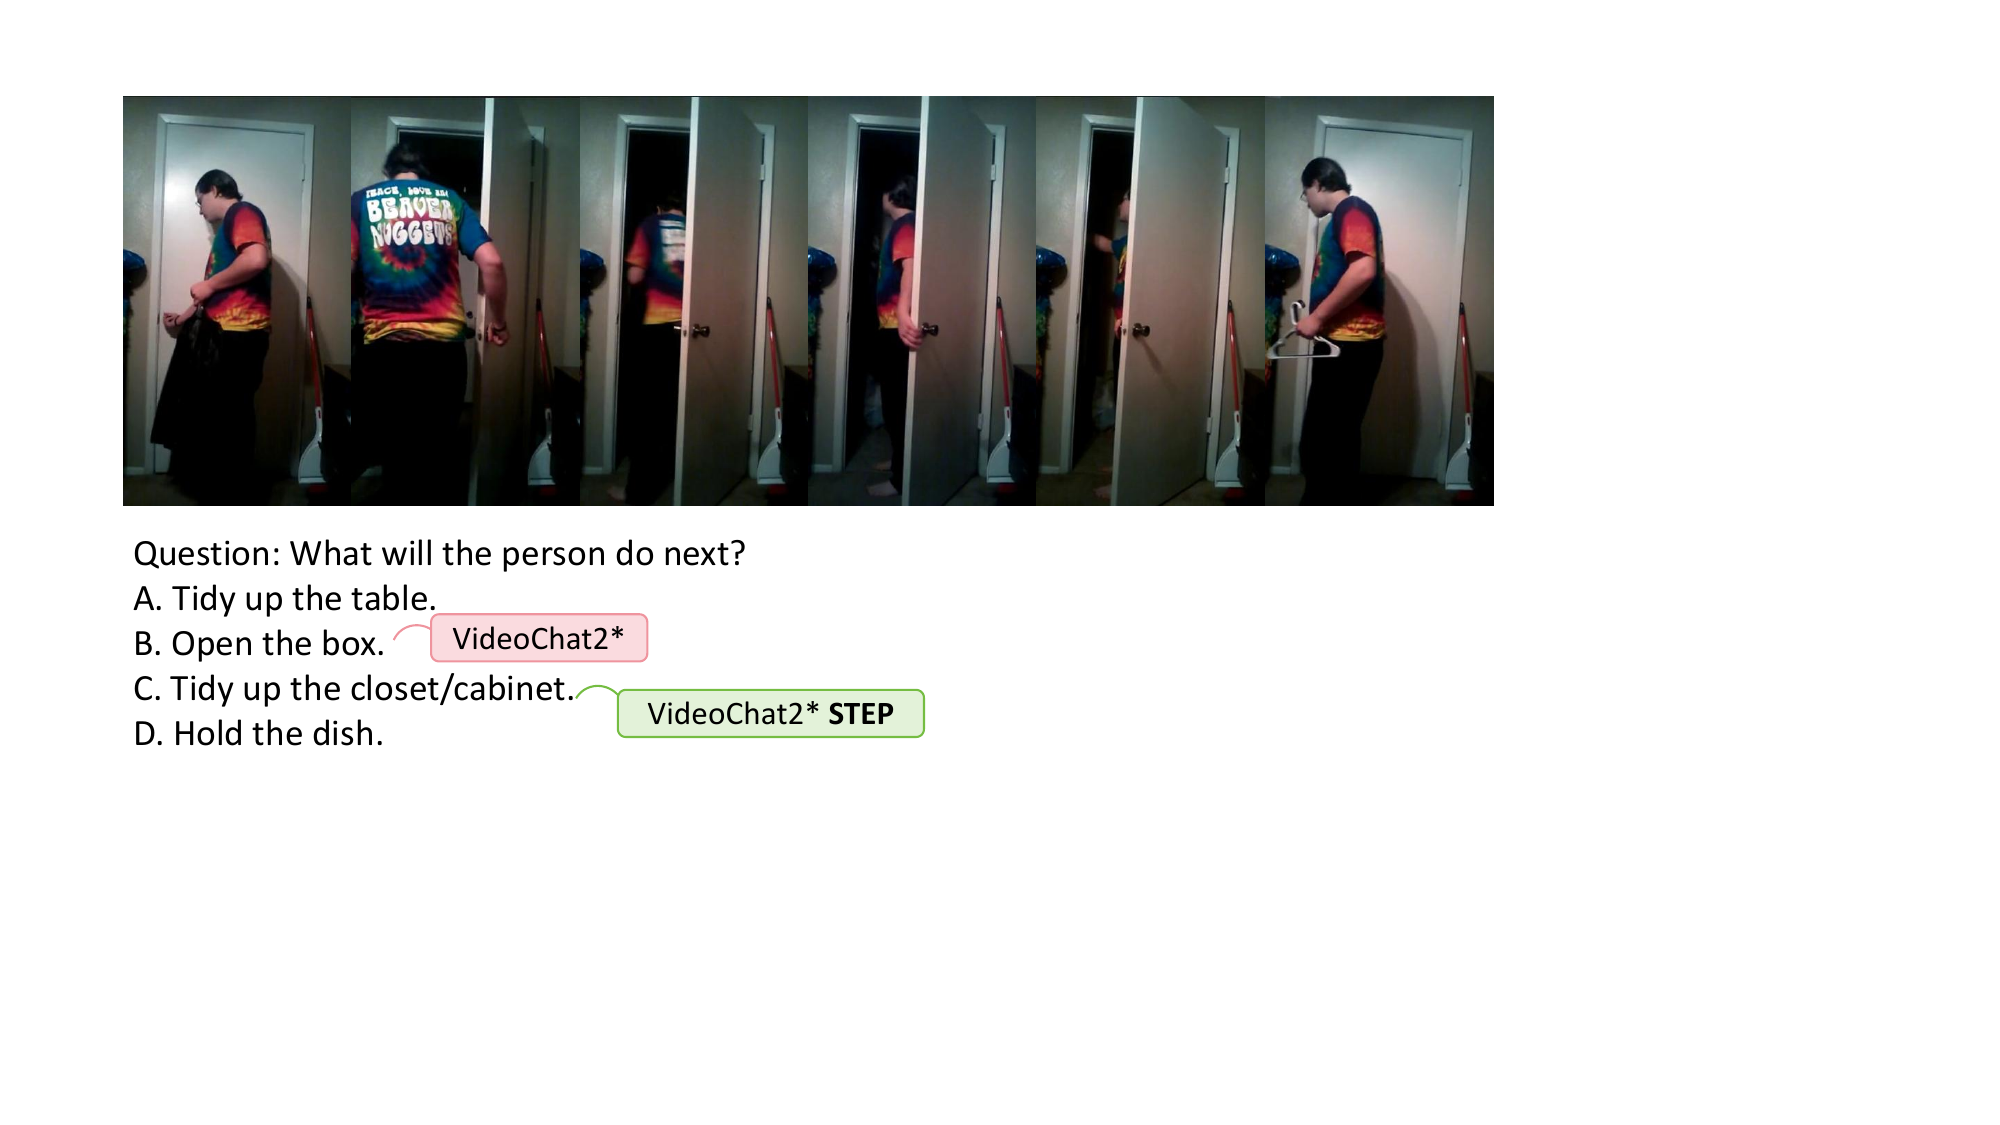}
    \caption{Qualitative examples of action prediction}
    \label{fig:eg4}
\end{figure}
\vspace{-3em}
\begin{figure}[h]
    \centering
    \vspace{1em}
    \includegraphics[width=\linewidth]{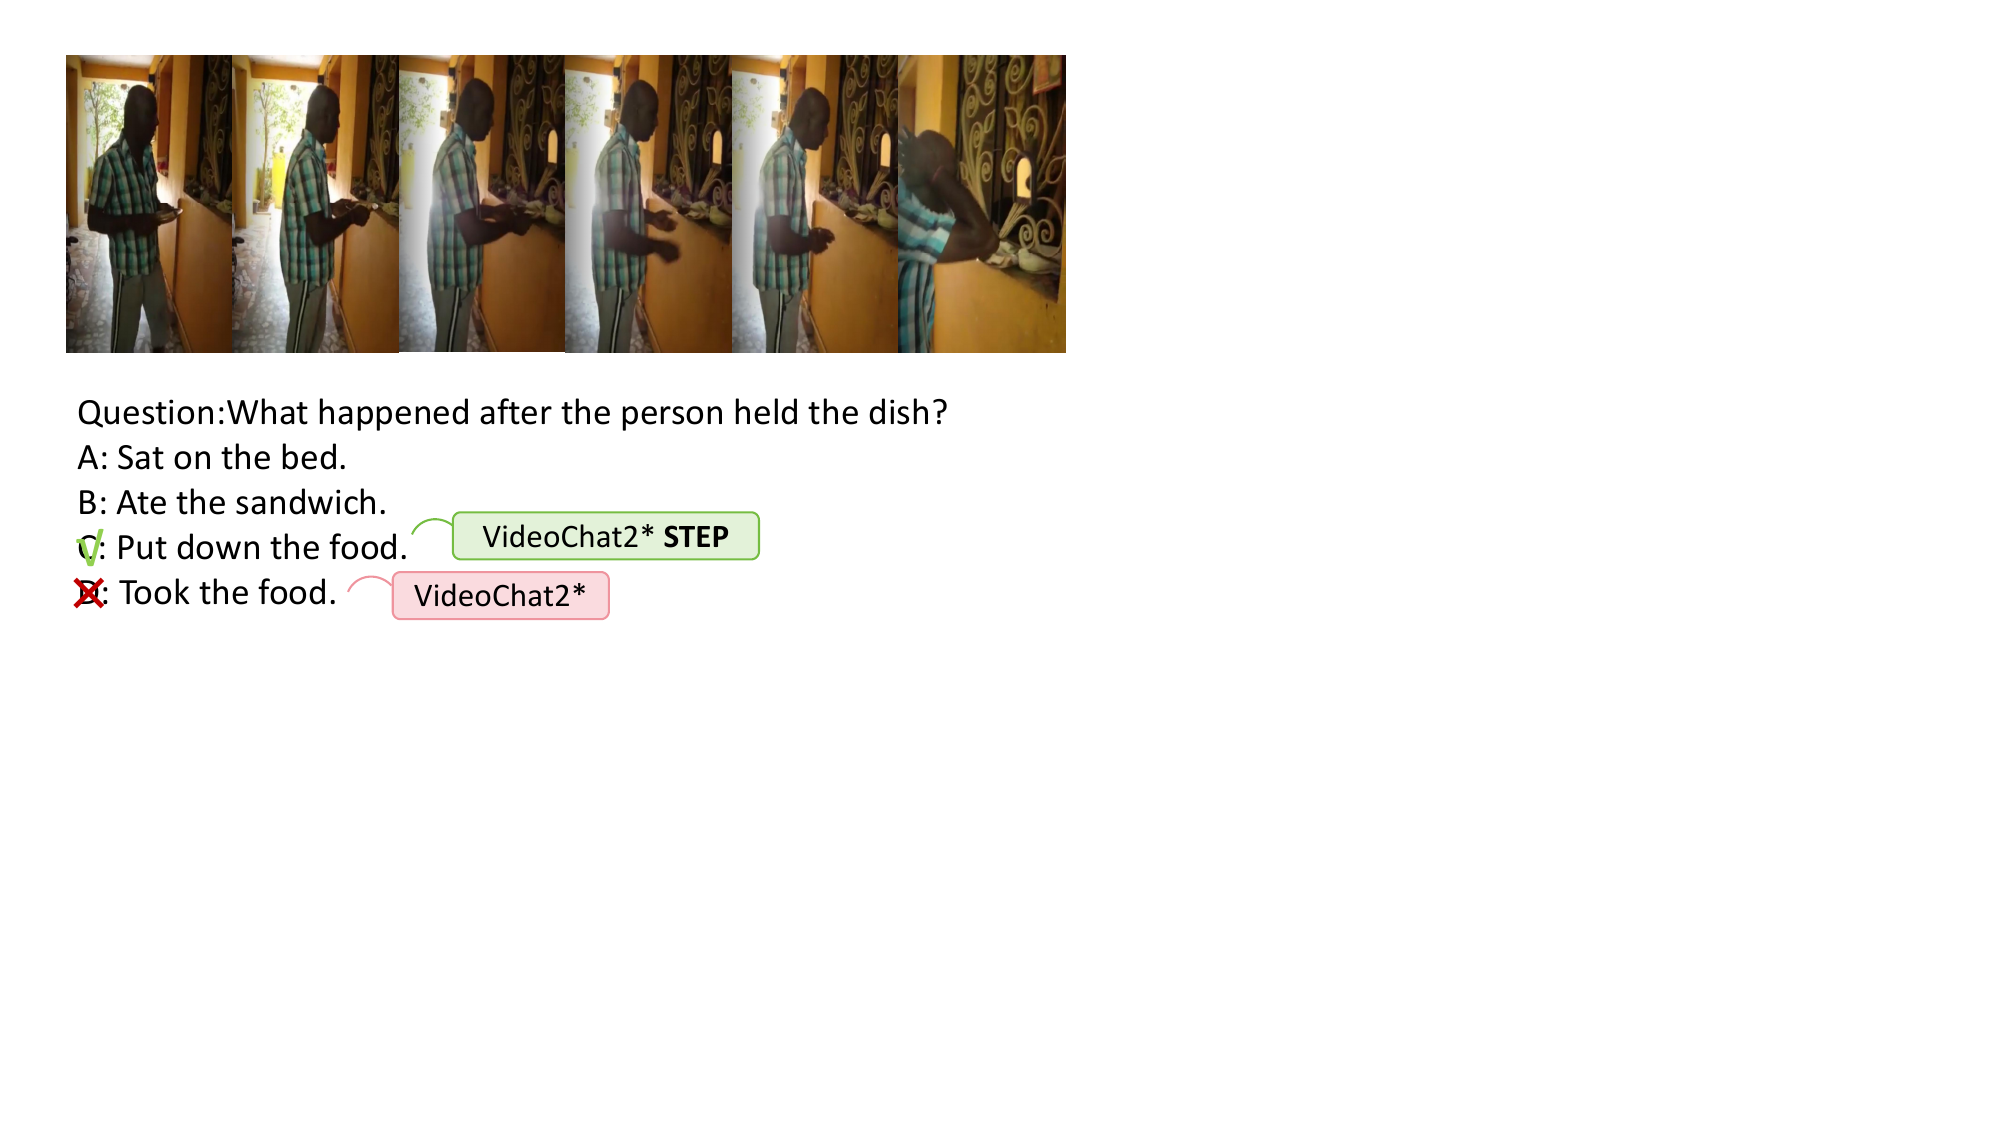}
    \caption{Qualitative examples of action sequence}
    \label{fig:eg1}
\end{figure}

\begin{figure}[H]
    \centering
    \includegraphics[width=\linewidth]{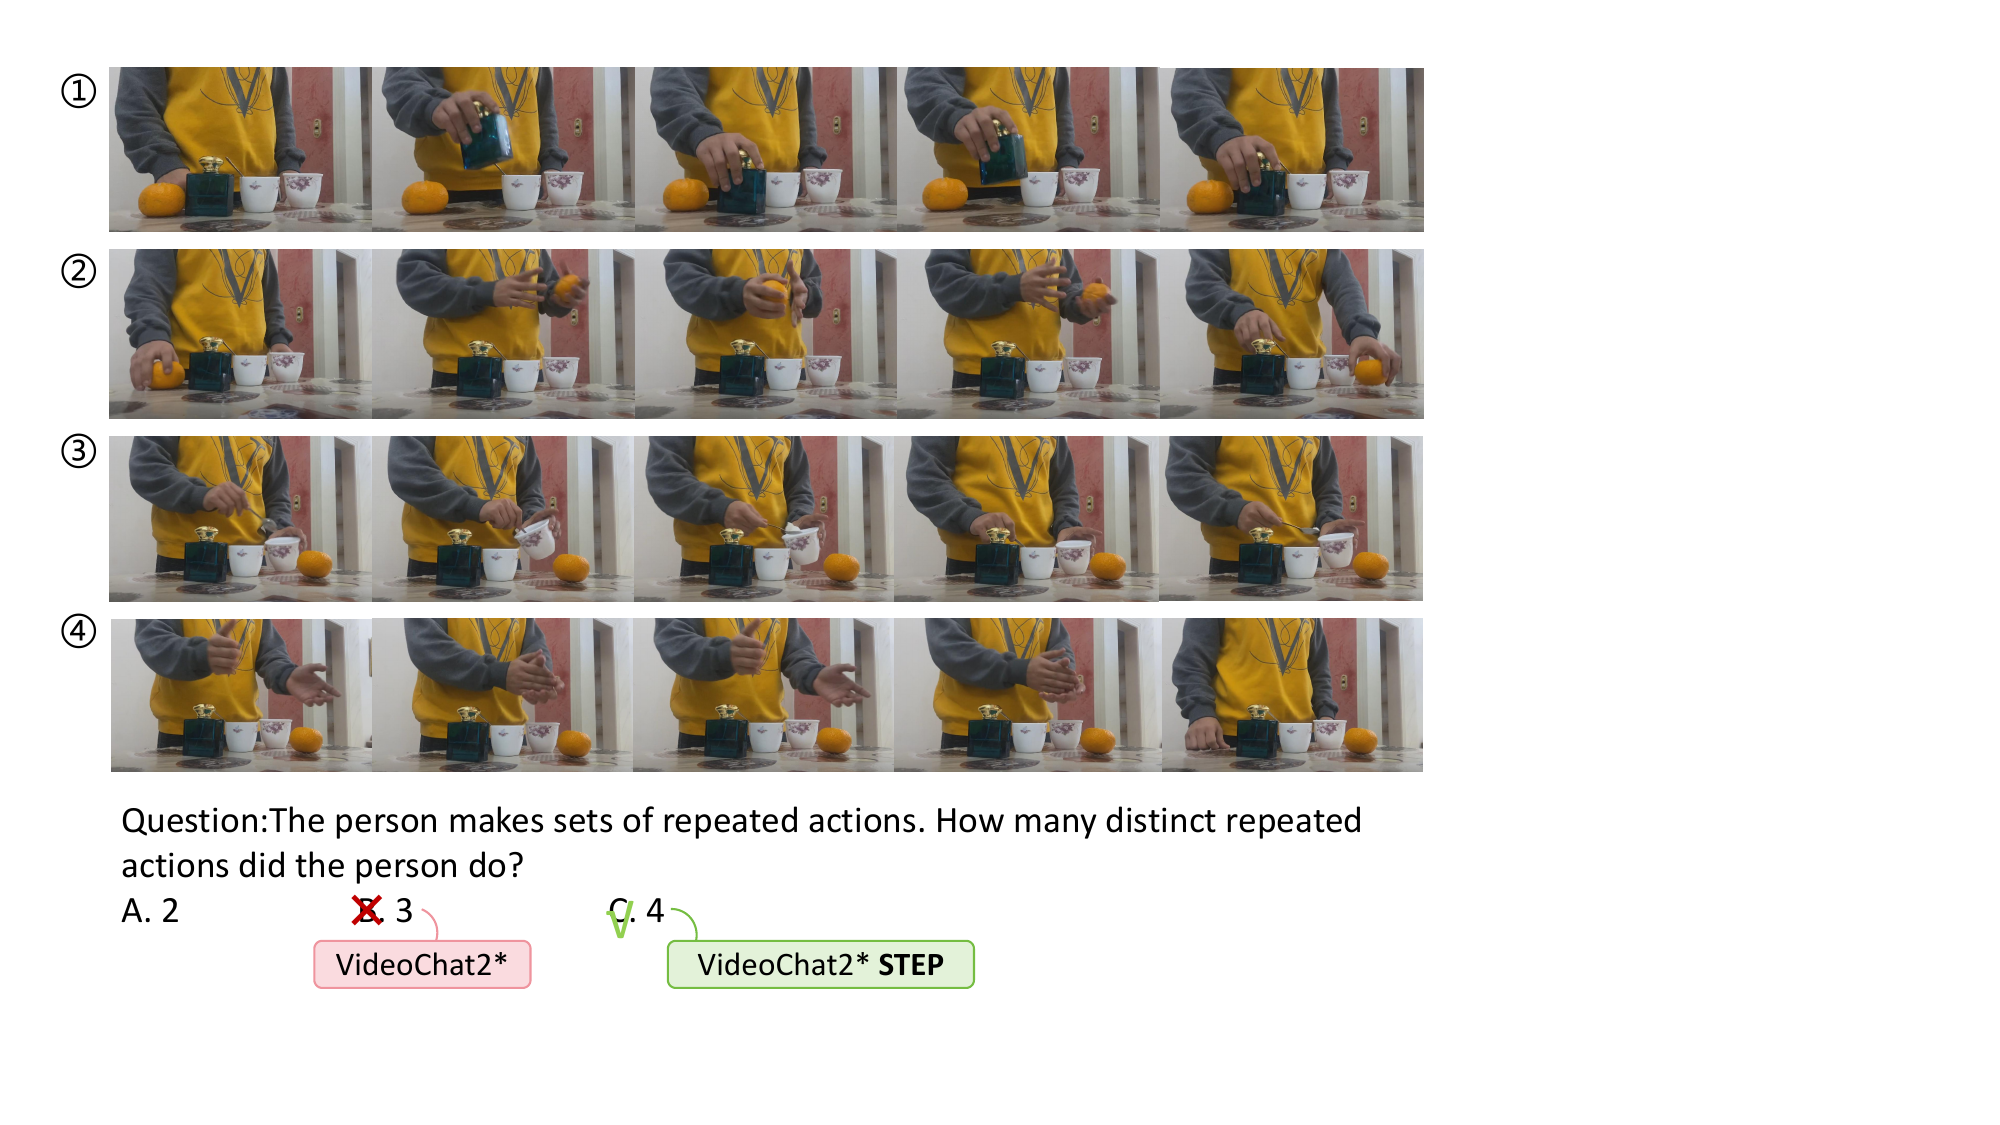}
    \caption{Qualitative examples of action count}
    \label{fig:eg2}
\end{figure}
